# Supplementary material for: Efficient Pose and Cell Segmentation using Column Generation
Source: arXiv:1612.00437 source file (2016-12-01)
Supplement: Supplementary file 1 [file cellSupplementaryInfo.tex]

\subsection{Cell segmentation experiments}
\label{suppl:cell}

We find a detection using Hungarian matching with centroid distance, and report matches between found segments and the manually labeled ground-truth (GT) regions based on area overlap. Unmatched GT regions are false negatives (FN), unmatched segmentation regions are false positives (FP). Results are reported in terms of precision P=TP/(TP+FP), recall R=TP/(TP+FN), and F-score F=2$\times$P$\times$R/(P+R).
